# Supplementary material for: Logicbreaks: A Framework for Understanding Subversion of Rule-based Inference
Source: arXiv:2407.00075 source file (2025-02-28)
Supplement: Supplementary file 2 [file q2_additional.tex]

\begin{figure}[ht]
\centering
% \includegraphics[width=0.5\linewidth]{images/exp_plots/exp2_additional/exp_theory_comp_plot_d128.pdf}
% \includegraphics[width=0.5\linewidth]{images/exp_plots/exp2_additional/exp_theory_comp_plot_d160.pdf}
% \includegraphics[width=0.5\linewidth]{images/exp_plots/exp2_additional/exp_theory_comp_plot_d192.pdf}
\begin{minipage}{0.33\linewidth}
    \centering
    \includegraphics[width=0.98\linewidth]{images/exp_plots/exp2_additional/exp_theory_comp_plot_128.pdf}
\end{minipage}%
\begin{minipage}{0.33\linewidth}
    \centering
    \includegraphics[width=0.98\linewidth]{images/exp_plots/exp2_additional/exp_theory_comp_plot_160.pdf}
\end{minipage}
\begin{minipage}{0.33\linewidth}
    \centering
    \includegraphics[width=0.98\linewidth]{images/exp_plots/exp2_additional/exp_theory_comp_plot_192.pdf}
\end{minipage}
\caption{Adversarial attacks designed for theoretical models partially translate to learned reasoners.
Appending a sufficiently large attack token \(u_{\msf{atk}}\) to two different input sequences causes even near-perfect reasoners to produce the same output.
This works by saturating the reasoner's softmax attention, where \(\kappa = \norm{u_{\msf{atk}}}_\infty\).}
\label{fig:q2_additional}
\end{figure}
