# Supplementary material for: Logicbreaks: A Framework for Understanding Subversion of Rule-based Inference
Source: arXiv:2407.00075 source file (2025-02-28)
Supplement: Supplementary file 3 [file q4_additional.tex]

\begin{figure}[htb]
\centering

% \includegraphics[width=0.5\linewidth]{images/exp_plots/exp4_additional/exp4_prob_plot_128.pdf}
% \includegraphics[width=0.5\linewidth]{images/exp_plots/exp4_additional/exp4_prob_plot_160.pdf}

\begin{minipage}{0.33\linewidth}
    \centering
    \includegraphics[width=0.98\linewidth]{images/exp_plots/exp4_additional/exp4_prob_plot_128.pdf}
\end{minipage}%
\begin{minipage}{0.33\linewidth}
    \centering
    \includegraphics[width=0.98\linewidth]{images/exp_plots/exp4_additional/exp4_prob_plot_160.pdf}
\end{minipage}
\begin{minipage}{0.33\linewidth}
    \centering
    \includegraphics[width=0.98\linewidth]{images/exp_plots/exp4_additional/exp4_prob_plot_192.pdf}
\end{minipage}
\caption{Near-perfect in-distribution learners fail to generalize when the rules have more hot bits.
We take near-perfect reasoners trained on rules drawn from the green band (\(0.2 \leq p_\alpha, p_\beta \leq 0.3\)) and test them on rules with antecedent and consequent probabilities \(p_\alpha ^{\msf{test}} = p_\beta ^{\msf{test}} = p^{\msf{test}}\) for \(p^{\msf{test}} \in \{0.1, 0.2, \ldots, 0.9\}\).
The reasoner accuracy decays when \(p^{\msf{test}} \gg 0.3\), but not when \(p^{\msf{test}} = 0.1\).}
\label{fig:q2_additional_prob}
\end{figure}

\begin{figure}[!htb]
\centering
% \includegraphics[width=0.5\linewidth]{images/exp_plots/exp4_additional/exp4_rules_plot_128.pdf}
% \includegraphics[width=0.5\linewidth]{images/exp_plots/exp4_additional/exp4_rules_plot_160.pdf}
\begin{minipage}{0.33\linewidth}
    \centering
    \includegraphics[width=0.98\linewidth]{images/exp_plots/exp4_additional/exp4_rules_plot_128.pdf}
\end{minipage}%
\begin{minipage}{0.33\linewidth}
    \centering
    \includegraphics[width=0.98\linewidth]{images/exp_plots/exp4_additional/exp4_rules_plot_160.pdf}
\end{minipage}
\begin{minipage}{0.33\linewidth}
    \centering
    \includegraphics[width=0.98\linewidth]{images/exp_plots/exp4_additional/exp4_rules_plot_192.pdf}
\end{minipage}
\caption{Near-perfect in-distribution reasoners fail to generalize when they see more rules than what they are trained on.
We take near-perfect reasoners trained on some number of rules drawn from the green band (\(16 \leq r \leq 64\)) and test them on distributions with \(r^{\msf{test}} \in \{8, 128, 256, 512\}\) number of rules.
For \(r^{\msf{test}} > 64\), the reasoning accuracy is lower than the near-perfect accuracy obtained for \(r^{\msf{test}} \leq 64\).}
\label{fig:q2_additional_rules}
\end{figure}
