# Supplementary material for: Logicbreaks: A Framework for Understanding Subversion of Rule-based Inference
Source: arXiv:2407.00075 source file (2025-02-28)
Supplement: Supplementary file 4 [file q5_additional.tex]

\begin{figure}[ht]
\centering
\begin{minipage}{0.5\linewidth}
    \centering
    \includegraphics[width=0.95\linewidth]{images/exp_plots/exp5_additional/ablations_heads.png}
\end{minipage}%
\begin{minipage}{0.5\linewidth}
    \centering
    \includegraphics[width=0.95\linewidth]{images/exp_plots/exp5_additional/ablations_layers.png}
\end{minipage}
\caption{Ablations on the number of heads \(H\) and the number of layers \(L\) for learning with \(n = 32\) propositions. When \(H = 1\) heads and \(L \in \{1, 2, 4, 8\}\) layers, the reasoning performance improves as \(L\) increases for embedding dimension \(d = 64\) but remains unchanged for \(d = 32\). Surprisingly and in contrast, when \(L = 1\) layers and \(H \in \{1, 2, 4, 8\}\) heads, the reasoning performance drops as \(H\) increases for \(d = 64\) and remains unchanged for \(d = 32\).}
\label{fig:q5_additional_ablations}
\end{figure}
