# Supplementary material for: Logicbreaks: A Framework for Understanding Subversion of Rule-based Inference
Source: arXiv:2407.00075 source file (2025-02-28)
Supplement: Supplementary file 5 [file additional_experiments.tex]

\section{Additional Experiments}
\label{sec:additional_experiments}


\subsection{Ablations on Model Parameters}
\label{sec:appendix_model_params}

% \input{figures/q5_additional}

\subsection{Additional Plots for the Theoretical Attack Experiments}
\label{sec:appendix_theory_attack}

\input{figures/q2_additional}

\subsection{Additional Plots for the Out-of-Distribution Robustness Experiments}
\label{sec:appendix_ood}

\input{figures/q4_additional}
